# Supplementary material for: Performance Impact of Memory Channels on Sparse and Irregular Algorithms
Source: arXiv:1910.03679 source file (2019-10-08)
Supplement: Supplementary file 1 [file appendix.tex]

\begin{figure}[t]

 \centering
 \subfloat[\PR]{
  \includegraphics[width=\columnwidth]{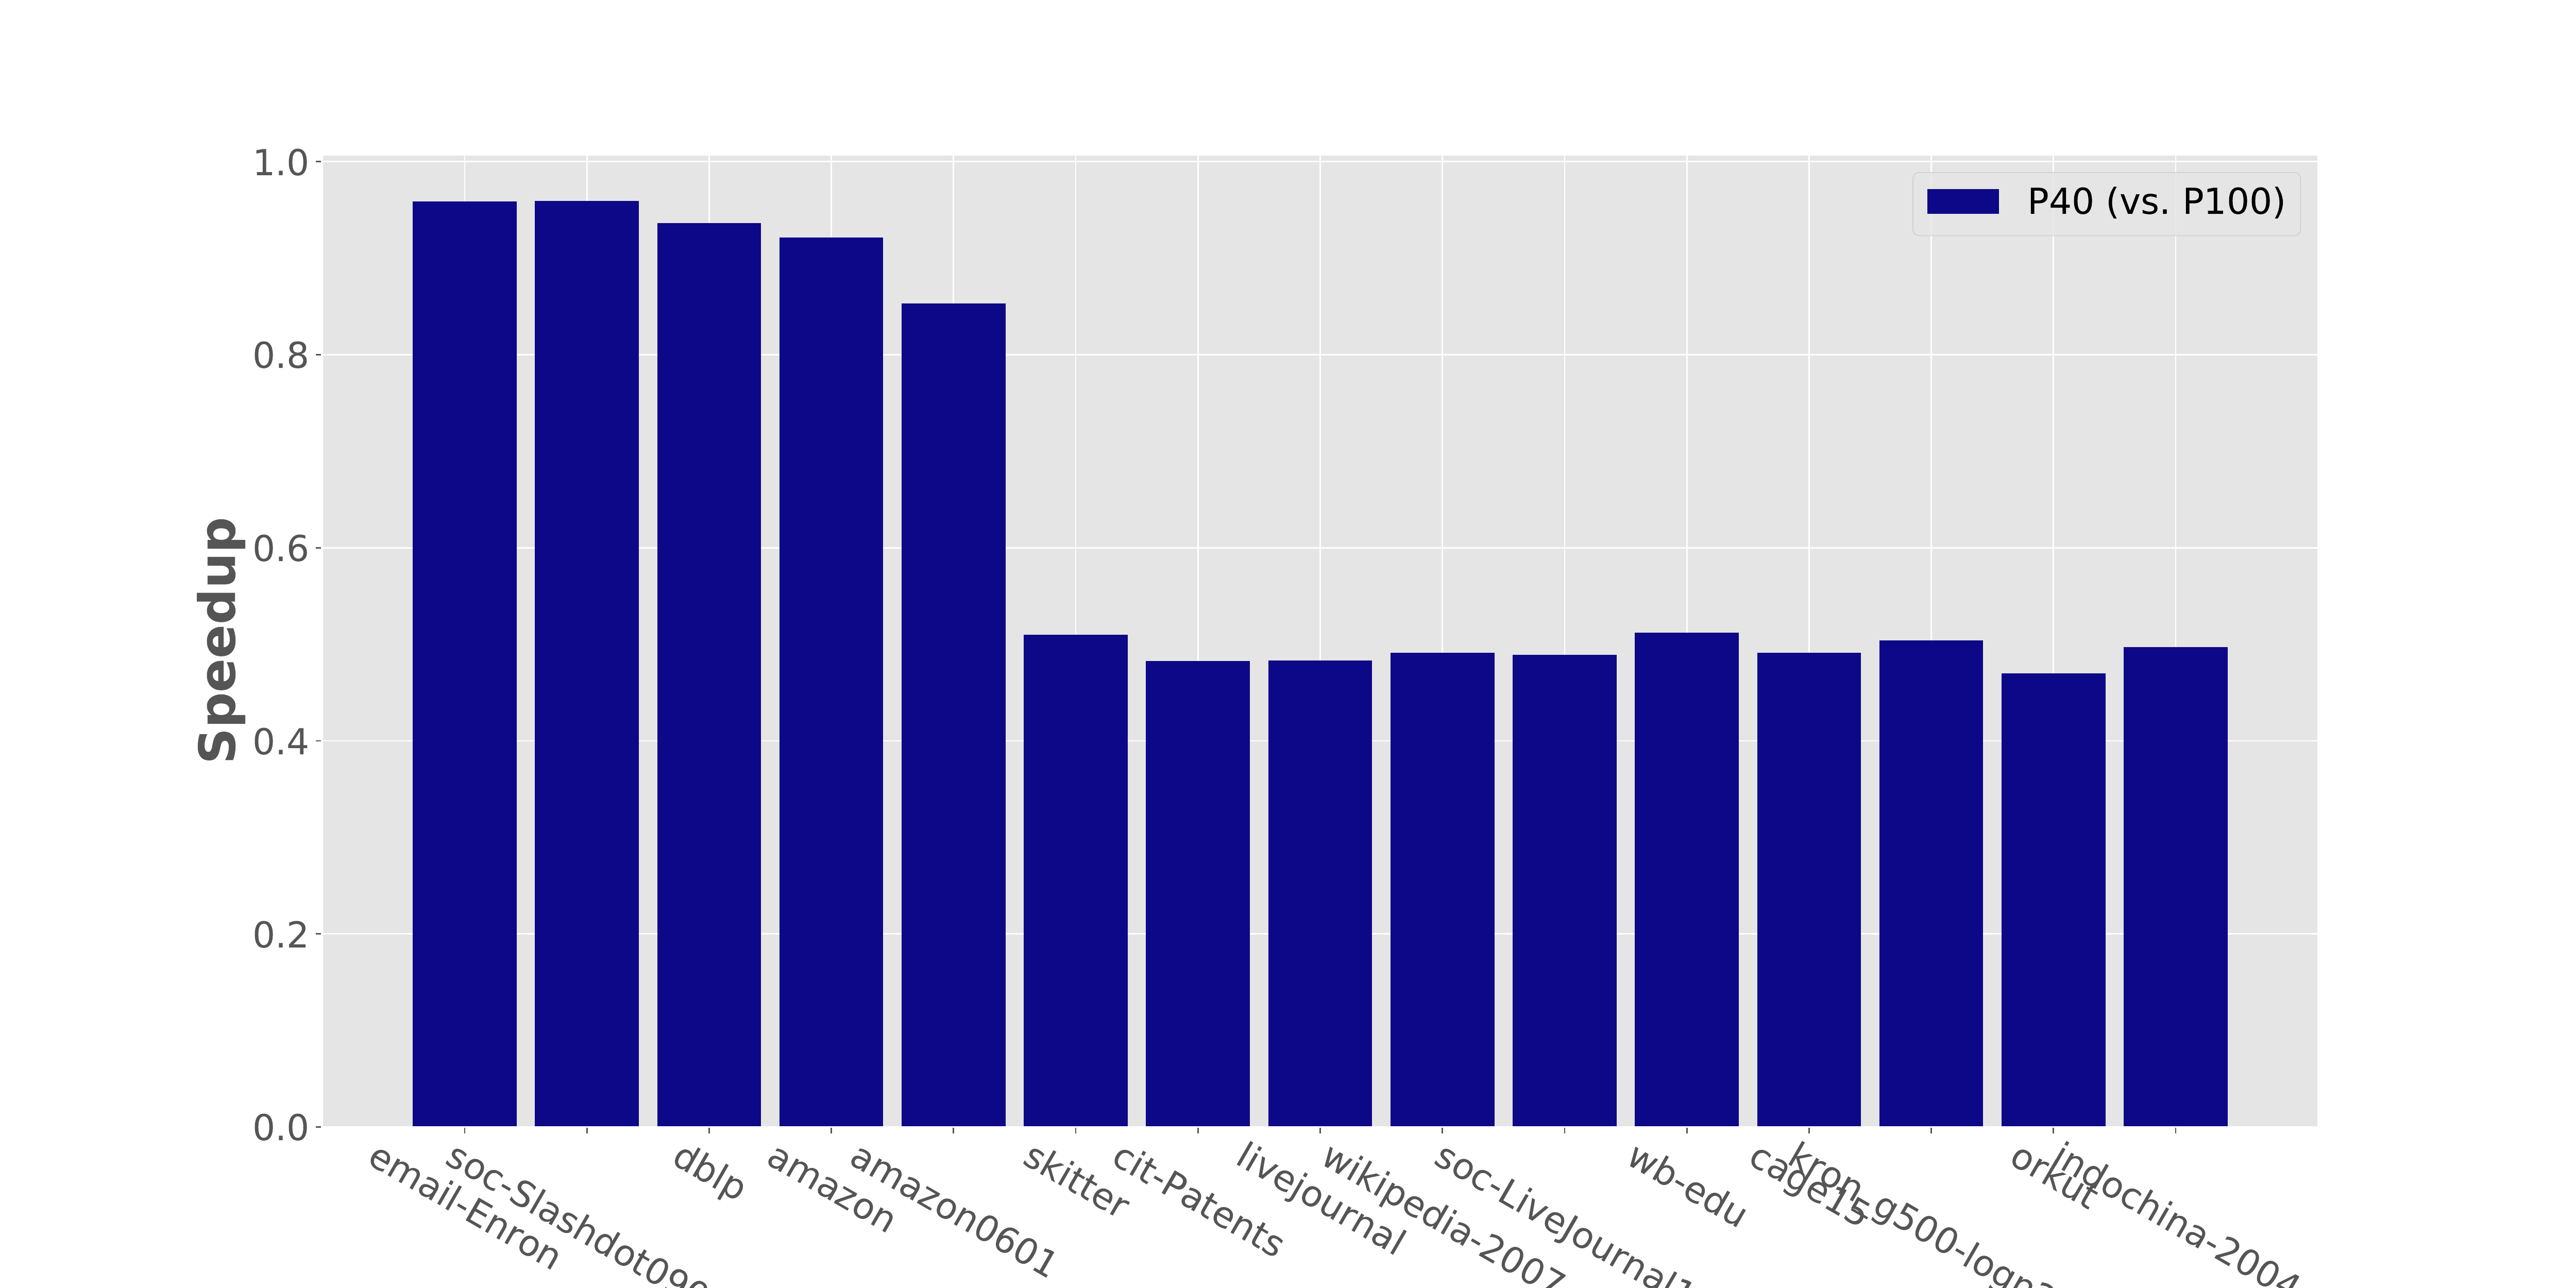}}
 \vspace{-0.3cm}

 \subfloat[\SSSP]{
   \includegraphics[width=\columnwidth]{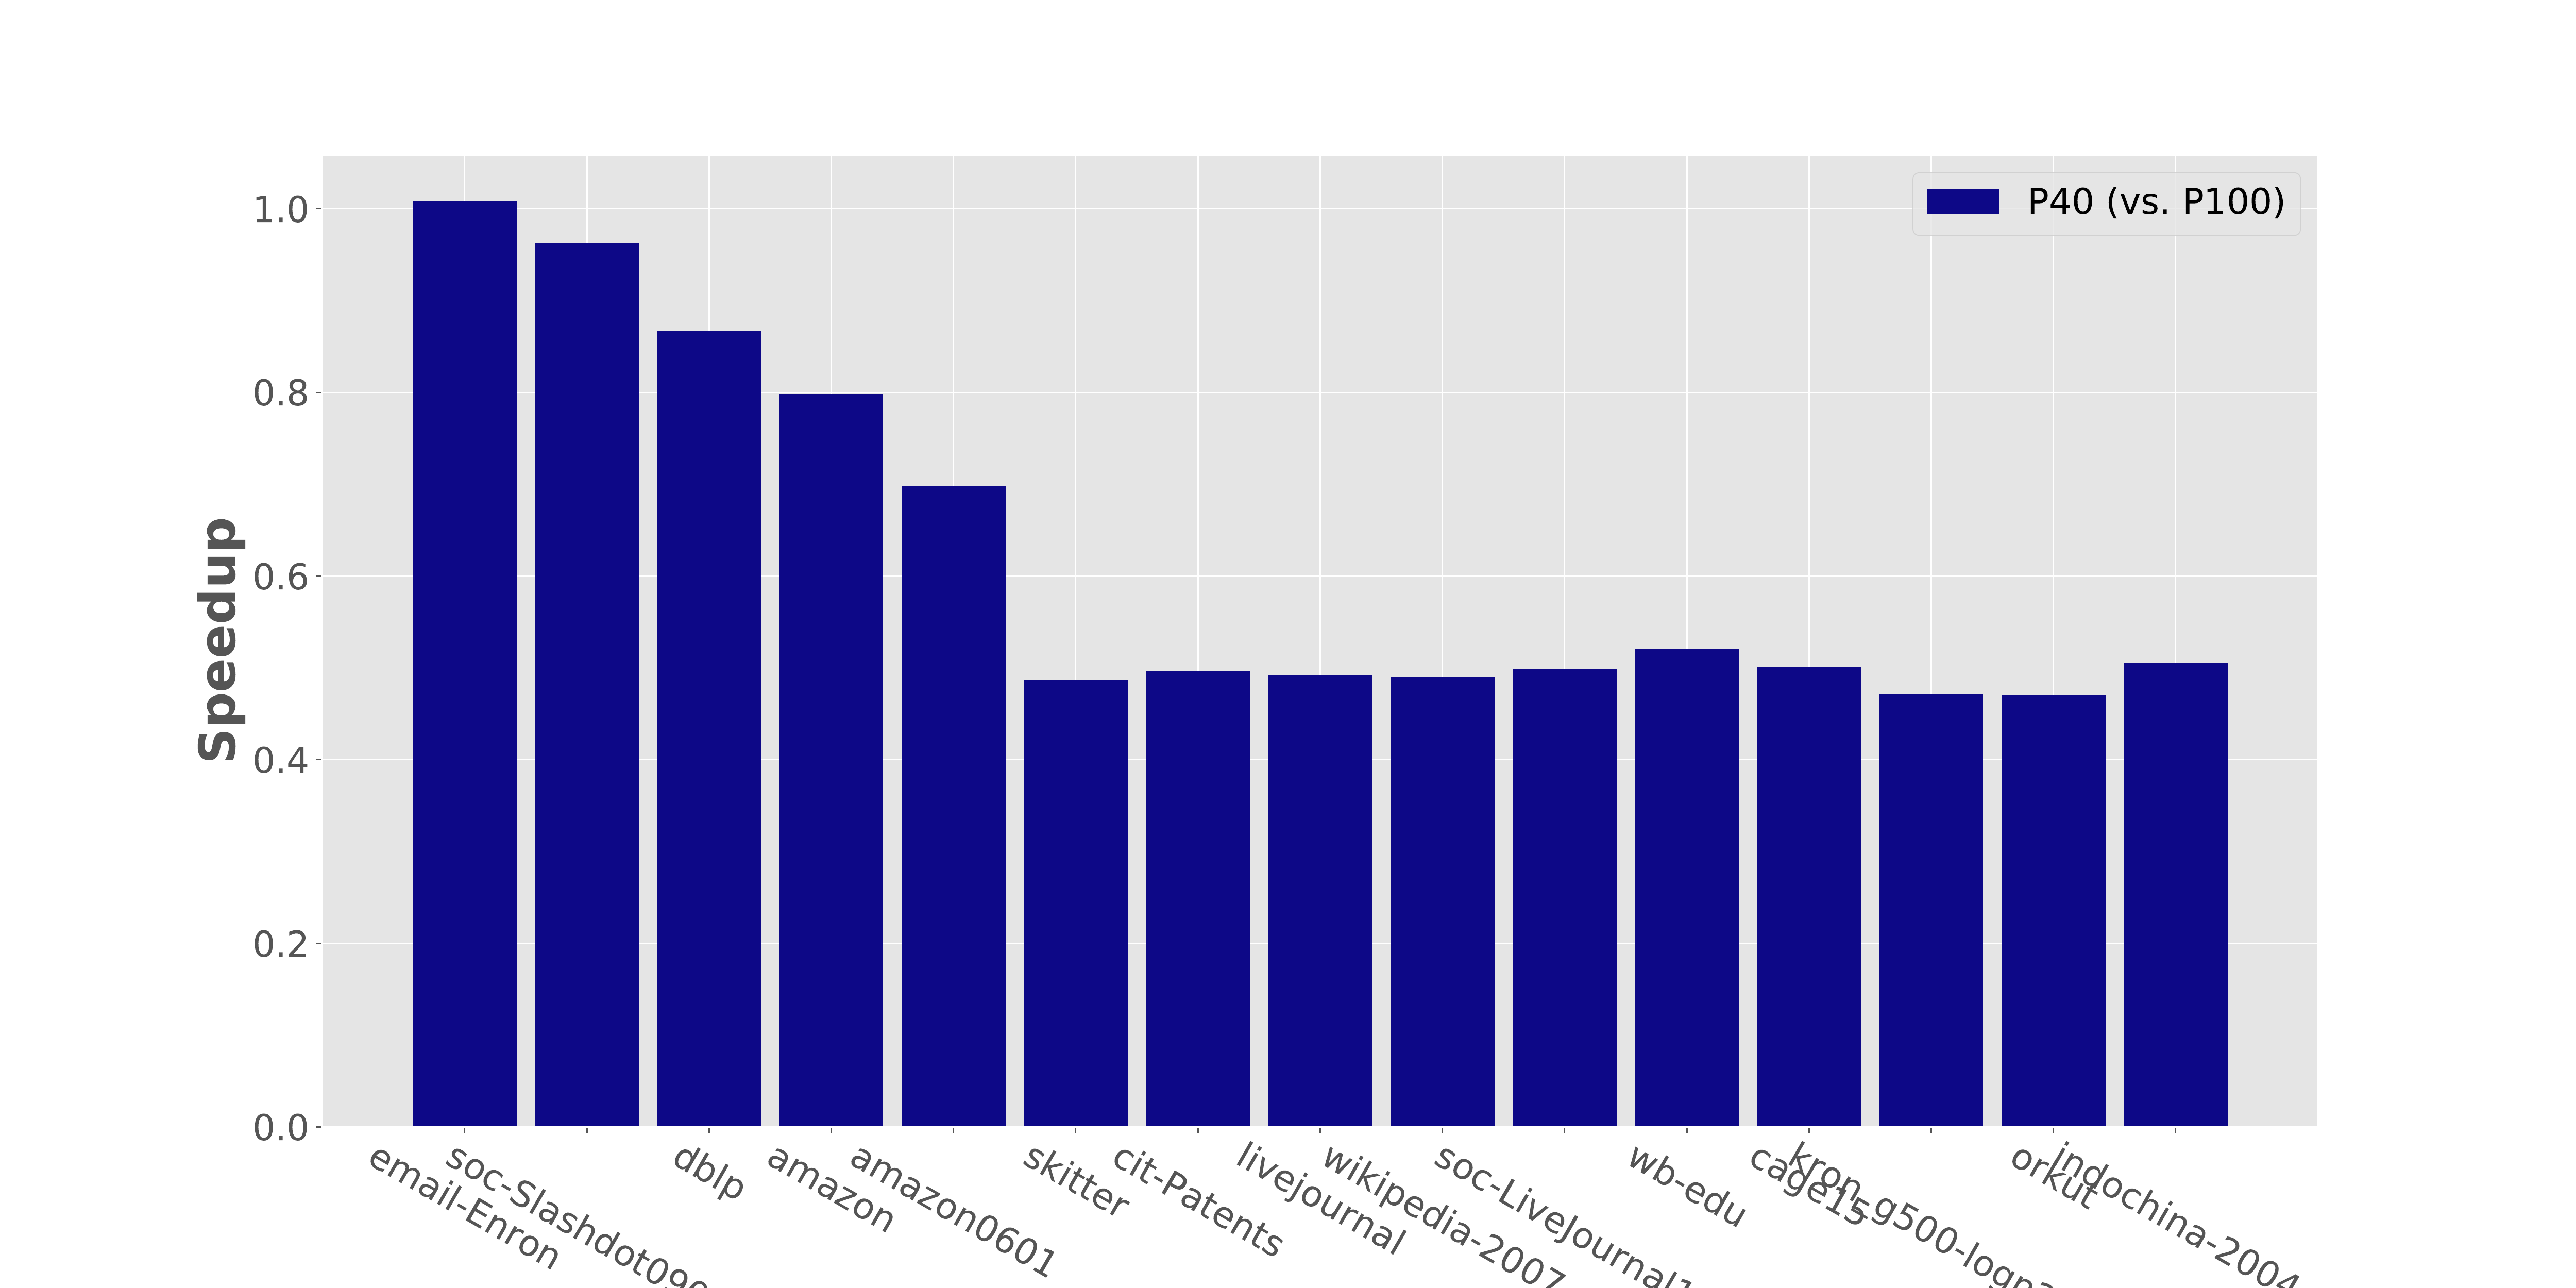}}
 %\vspace{-0.3cm}

   \caption{Speedup for \PR and \SSSP using \NVG framework for the GPU.  Execution times are normalized to the execution time of the P100 GPU with HBM memory. See Table \ref{tab:graphs} for details about inputs used.}
 \label{fig:nvgraph}	
 
 \end{figure}
